# Supplementary material for: An Unsupervised Domain Adaptive Approach for Multimodal 2D Object Detection in Adverse Weather Conditions
Source: arXiv:2203.03568 source file (2022-03-07)
Supplement: Supplementary file 1 [file supplementary.tex]

In synthetic data, all modalities suffer from domain change: image style and objects texture are different while pointclouds are less noisy than their real counterparts.
 
 %@inproceedings{mees2016choosing,
%  title={Choosing Smartly: Adaptive Multimodal Fusion for Object Detection in Changing Environments},
%  author={Mees, Oier and Eitel, Andreas and Burgard, Wolfram},
%  booktitle=IEEE_IROS,
%  pages={151--156},
%  year={2016},
%  xorganization={IEEE}
%}

@article{He2020DomainAO,
  title={Domain Adaptive Object Detection via Asymmetric Tri-way Faster-RCNN},
  author={Zhenwei He and L. Zhang},
  journal={ArXiv},
  year={2020},
  volume={abs/2007.01571}
}

The dataset contains 5.5k frames captured in clear weather, 1k captured in dense fog, 1k in light fog and 4k in snow or rain conditions.

\begin{table*}[h]%[bp]
\caption{Single Target Domain Adaptation Results.}
\setlength\tabcolsep{4.2pt}
\begin{center}
\scalebox{0.95}{
\begin{tabular}{lccc|>{\columncolor[gray]{0.95}} c|ccc|>{\columncolor[gray]{0.95}}c|ccc|>{\columncolor[gray]{0.95}}c|ccc|>{\columncolor[gray]{0.95}}c|ccc|>{\columncolor[gray]{0.95}}c}
	\toprule
  & \multicolumn{4}{c}{Clear}  & \multicolumn{4}{c}{Light Fog}  & \multicolumn{4}{c}{Dense Fog}  & \multicolumn{4}{c}{Snow}  & \multicolumn{4}{c}{Night}  \\
  \midrule
  & \rotatebox[origin=l]{90}{Car} & \rotatebox[origin=l]{90}{Person} & \rotatebox[origin=l]{90}{Cyclist} & \rotatebox[origin=l]{90}{mean} & \rotatebox[origin=l]{90}{Car} & \rotatebox[origin=l]{90}{Person} & \rotatebox[origin=l]{90}{Cyclist} & \rotatebox[origin=l]{90}{mean} & \rotatebox[origin=l]{90}{Car} & \rotatebox[origin=l]{90}{Person} & \rotatebox[origin=l]{90}{Cyclist} & \rotatebox[origin=l]{90}{mean} & \rotatebox[origin=l]{90}{Car} & \rotatebox[origin=l]{90}{Person} & \rotatebox[origin=l]{90}{Cyclist} & \rotatebox[origin=l]{90}{mean} & \rotatebox[origin=l]{90}{Car} & \rotatebox[origin=l]{90}{Person} & \rotatebox[origin=l]{90}{Cyclist} & \rotatebox[origin=l]{90}{mean} \\
  \midrule
 Lidar Only & 57.2 & 45.1 & 34.9 & 00.0 & 51.5 & 14.2 & 0.2 & 00.0 & 27.6 & 20.1 & 8.1 & 00.0 & 51.4 & 43.2 & 9.3 & 00.0 & 61.6 & 50.0 & 20.2 & 00.0 \\
 RGB Only & 79.8 & 75.5 & 67.7 & 00.0 & 82.2 & 39.2 & 0.2 & 00.0 & 70.9 & 53.3 & 15.3 & 00.0 & 75.5 & 77.3 & 19.5 & 00.0 & 46.9 & 52.6 & 16.0 & 00.0 \\
 \midrule
 MultiModal \cite{bijelic2019seeing} & 81.8 & 74.8 & 69.8 & 00.0 & 84 & 38.2 & 5.8 & 00.0 & 71.2 & 50 & 11.3 & 00.0 & 78 & 78.4 & 20.8 & 00.0 & 59.3 & 63.4 & 22.7 & 00.0 \\
 \midrule
 CSD & 00.0 & 00.0 & 00.0 & 00.0 & 00.0 & 00.0 & 00.0 & 00.0 & 00.0 & 00.0 & 00.0 & 00.0 & 00.0 & 00.0 & 00.0 & 00.0 & 00.0 & 00.0 & 00.0 & 00.0 \\
 ADDA & 00.0 & 00.0 & 00.0 & 00.0 & 83.5 & 38.6 & 2.5 & 00.0 & 77.3 & 54.5 & 14.8 & 00.0 & 75.1 & 77.2 & 12.7 & 00.0 & 54.3 & 57.8 & 22.5 & 00.0 \\
 CyCADA & 00.0 & 00.0 & 00.0 & 00.0 & 00.0 & 00.0 & 00.0 & 00.0 & 00.0 & 00.0 & 00.0 & 00.0 & 00.0 & 00.0 & 00.0 & 00.0 & 00.0 & 00.0 & 00.0 & 00.0 \\
 \midrule
 Ours & 81.8 & 74.8 & 69.8 & 00.0 & 86.3 & 45.7 & 2.3 & 00.0 & 82.6 & 61.4 & 13.2 & 00.0 & 81.6 & 80.3 & 25.3 & 00.0 & 68.8 & 67.7 & 40.5 & 00.0 \\
 \midrule
 Oracle & 84.6 & 76.8 & 74.3 & 00.0 & 93 & 52.5 & 4 & 00.0 & 92.8 & 74.6 & 15 & 00.0 & 87 & 82 & 29.6 & 00.0 & 81.2 & 74.7 & 49.3 & 00.0 \\
\bottomrule
\end{tabular}
}
\end{center}
\end{table*}
